# Supplementary material for: Convergence Rates of Stochastic Zeroth-order Gradient Descent for \L ojasiewicz Functions
Source: arXiv:2210.16997 source file (2023-04-19)
Supplement: Supplementary file 2 [file appendix.tex]

\begin{proof}

    It is succifient to consider the estimator at $x = 0$. 
    Since $f$ is $L$-smooth, its gradient $\nabla f (x)$ is Lipschitz and thus absolutely continuous. Thus for any $v_i$, $ v_i^\top \nabla^2 f (x) v_i $ exists almost everywhere and $ v_i^\top \nabla^2 f (x) v_i $ is integrable. 
    
    Thus by Taylor's theorem, we have, for any fixed $v_i$,  
    \begin{align*} 
        f (\delta v_i) 
        = 
        f (0) + \delta v_i^\top \nabla f (0) + 
        % \delta^2 
        \int_{0}^{\delta} v_i^\top \nabla^2 f (t) v_i (\delta-t) \,dt. 
    \end{align*} 
    To avoid notational clutter, write $ I_i (\delta) := \int_{0}^{\delta} v_i^\top \nabla^2 f (t) v_i (\delta-t) \,dt $. 
    Thus it holds that 
    \begin{align*} 
        \E \[ \left\| \wh{\nabla}  f_k^\delta (0) \right\|^2 \] 
        =& \;  
        \E \[ \left\| \sum_{i=1}^k \frac{n}{2\delta k} \( f (\delta v_i) - f (-\delta v_i) \) v_i \right\|^2 \] \\ 
        =& \; 
        \E \[ \sum_{i=1}^k \left\| \frac{n}{2\delta k} \( f (\delta v_i) - f (-\delta v_i) \) v_i \right\|^2 \] \\ 
        =& \; 
        \E \[ \sum_{i=1}^k \nabla f (0)^\top v_i v_i^\top \nabla f (0) \] + \E \[ \( I_i (\delta) \)^2 \], 
    \end{align*} 
    where (\ref{??}) 

\end{proof}
